# Supplementary material for: A Systematic Study of Joint Representation Learning on Protein Sequences and Structures
Source: arXiv:2303.06275 source file (2023-10-18)
Supplement: Supplementary file 1 [file 06_appendix.tex]

\section{Experimental Details}

\subsection{Dataset Statistics}

\begin{table}[!h]
    \centering
    \caption{Dataset statistics for downstream tasks.}
    \label{tab:dataset}
    \begin{adjustbox}{max width=0.6\linewidth}
        %\footnotesize
        \begin{tabular}{lccc}
            \toprule
            \multirow{2}{*}{\bf{Dataset}} &
            \multicolumn{3}{c}{\bf{\# Proteins}}\\
            & \bf{\# Train} & \bf{\# Validation} & \bf{\# Test}\\
            \midrule
            \bf{Enzyme Commission} & 15,550 & 1,729 & 1,919 \\
            \bf{Gene Ontology} & 29,898 & 3,322 & 3,415 \\
            \bf{Fold Classification - \emph{Fold}} & 12,312 & 736 & 718 \\
            \bf{Fold Classification - \emph{Superfamily}} & 12,312 & 736 & 1,254 \\
            \bf{Fold Classification - \emph{Family}} & 12,312 & 736 & 1,272 \\
            \bf{Reaction Classification} & 29,215 & 2,562 & 5,651 \\
            \bottomrule
        \end{tabular}
    \end{adjustbox}
\end{table}

Dataset statistics of downstream tasks are summarized in Table~\ref{tab:dataset}.
Details are introduced as follows.

\paragraph{Enzyme Commission and Gene Ontology.}
Following DeepFRI~\citep{gligorijevic2021structure}, the EC numbers are selected from the third and fourth levels of the EC tree, forming 538 binary classification tasks, while the GO terms with at least 50 and no more than 5000 training samples are selected. The non-redundant sets are partitioned into training, validation and test sets according to the sequence identity.
We retrieve all protein chains from PDB with the code in their codebase and remove those with obsolete pdb ids, so the statistics will be slightly different from that in the original paper.

\paragraph{Fold Classification.}
We directly use the dataset in~\citet{hermosilla2020intrinsic}, which consolidated 16,712 proteins with 1,195 different folds from the SCOPe 1.75 database~\citep{murzin1995scop}.

\paragraph{Reaction Classification.}
The dataset comprises 37,428 proteins categorized into 384 reaction classes. 
The split methods are described in~\citet{hermosilla2020intrinsic}, where they cluster protein chains via sequence similarities and ensure that protein chains from the same cluster are in the same split. 

\subsection{Evaluation Metrics}
\label{sec:app_eval}
Now we introduce the details of evaluation metrics for EC and GO prediction.
These two tasks aim to answer the question: whether a protein has some particular functions, which can be seen as multiple binary classification tasks.

The first metric, protein-centric maximum F-score F\textsubscript{max}, is defined by first calculating the precision and recall for each protein and then taking the average score over all proteins.
More specifically, for a given target protein $i$ and a decision threshold $t\in[0,1]$, the precision and recall are computed as:
\begin{align}
    \text{precision}_i(t)=\frac{\sum_f \mathbbm{1}[f\in P_i(t) \cap T_i]}{\sum_f \mathbbm{1}[f\in P_i(t)]},
\end{align}
and
\begin{align}
    \text{recall}_i(t)=\frac{\sum_f \mathbbm{1}[f\in P_i(t) \cap T_i]}{\sum_f \mathbbm{1}[f\in T_i]},
\end{align}
where $f$ is a function term in the ontology, $T_i$ is a set of experimentally determined function terms for protein $i$, $P_i(t)$ denotes the set of predicted terms for protein $i$ with scores greater than or equal to $t$ and $\mathbbm{1}[\cdot]\in\{0,1\}$ is an indicator function that is equal to $1$ \emph{iff} the condition is true.

Then, the average precision and recall over all proteins at threshold $t$ is defined as:
\begin{align}
    \text{precision}(t)=\frac{1}{M(t)}\sum_{i} \text{precision}_i(t),
\end{align}
and
\begin{align}
    \text{recall}(t)=\frac{1}{N}\sum_{i} \text{recall}_i(t),
\end{align}
where we use $N$ to denote the number of proteins and $M(t)$ to denote the number of proteins on which at least one prediction was made above threshold $t$, \emph{i.e.}, $|P_i(t)|>0$.

Combining these two measures, the maximum F-score is defined as the maximum value of F-measure over all thresholds.
That is,
\begin{align}
    \text{F\textsubscript{max}}=
    \max_t\left\{\frac{2\cdot \text{precision}(t)\cdot \text{recall}(t)}{\text{precision}(t)+ \text{recall}(t)}\right\}.
\end{align}

The second metric, pair-centric area under precision-recall curve AUPR\textsubscript{pair}, is defined as the average precision scores for all protein-function pairs, which is exactly the micro average precision score for multiple binary classification.

\subsection{Implementation Details}
\label{sec:app_impl}
In this subsection, we describe implementation details of all baselines and our methods.
For all models, the outputs will be fed into a three-layer MLP to make final prediction.
The dimension of hidden layers in the MLP is equal to the dimension of model outputs.

% \paragraph{Sequence-based encoders~\cite{tape2019}.}

% \paragraph{Pretrained language models~\cite{rives2021biological}.}

\paragraph{CNN~\citep{shanehsazzadeh2020transfer}.} Following the finding in~\citet{shanehsazzadeh2020transfer}, we employ a convolutional neural network (CNN) to encode protein sequences. Specifically, 2 convolutional layers with 1024 hidden dimensions and kernel size 5 constitute this baseline model. 

\paragraph{ResNet~\citep{tape2019}.} We also adopt a deep CNN model, \emph{i.e.}, the ResNet for protein sequences proposed by~\citet{tape2019}, in our benchmark. This model is with 12 residual blocks and 512 hidden dimensions, and it uses the GELU~\citep{hendrycks2016gaussian} activation function.

\paragraph{LSTM~\citep{tape2019}.} The bidirectional LSTM model proposed by~\citet{tape2019} is another baseline for protein sequence encoding. It is composed of three bidirectional LSTM layers with 640 hidden dimensions.

\paragraph{Transformer~\citep{tape2019}.} The self-attention-based Transformer encoder~\citep{vaswani2017attention} is a strong model in natural language processing (NLP), \citet{tape2019} adapts this model into the field of protein sequence modeling. We also adopt it as one of our baselines. This model has a comparable size with BERT-Small~\citep{devlin2018bert}, which contains 4 Transformer blocks with 512 hidden dimensions and 8 attention heads, with activation GELU~\citep{hendrycks2016gaussian}.  

\paragraph{GCN~\citep{kipf2017semi}.} We take GCN as a baseline to encode the residue graph derived by our graph construction scheme. We adopt the implementation in TorchDrug~\citep{zhu2022torchdrug}, where 6 GCN layers with the hidden dimension of 512 are used. We run the results of GCN on EC and GO by ourselves and take its results on Fold and Reaction classification from~\citet{hermosilla2020intrinsic}.

\paragraph{GAT~\citep{velickovic2018graph}.} We adopt another popular graph neural network, GAT, as a structure-based baseline. We follow the implementation in TorchDrug and use 6 GAT layers with the hidden dimension of 512 and 1 attention head per layer for encoding. The results on EC, Fold and Reaction classification are based on our runs, and the results on GO are taken from~\citet{wang2021lm}.

% \paragraph{GCN~\cite{kipf2017semi}, GAT~\cite{velickovic2018graph}.}
% We adopt the implementation of the two graph neural networks in TorchDrug~\cite{zhu2022torchdrug} and run GCN for EC, GO prediction and GAT for EC, Fold and Reaction classification.
% @Minghao

\paragraph{GVP~\citep{jing2021equivariant}.} The GVP model~\citep{jing2021equivariant} is a decent protein structure encoder. It iteratively updates the scalar and vector representations of a protein, and these representations possess the merit of invariance and equivariance. In our benchmark, we evaluate this baseline method following the official source code. In specific, 3 GVP layers with 32 feature dimensions (20 scalar and 4 vector channels) constitute the GVP model. 

\paragraph{3DCNN\_MQA~\citep{derevyanko2018deep}.}
We implement the 3DCNN model from the paper~\citep{derevyanko2018deep} with a box width of 40.0 and input resolution of $120\times120\times 120$.
The model has 6 residual blocks and 128 hidden dimensions with ELU activation function.

\paragraph{GraphQA~\citep{baldassarre2021graphqa}.}
Following hyperparameters in the original paper, we construct residue graphs based on bond and spatial information and re-implement the graph neural network.
The best model has 4 layers with 128 node features, 32 edge features and 512 global features.

\paragraph{New IEConv~\citep{anonymous2022contrastive}.}
Since the code for New IEConv has not been made public when the paper is written, we reproduce the method according to the description in the paper and achieve similar results on Fold and Reaction classification tasks.
Then, we evaluate the method on EC and GO prediction tasks with the default hyperparameters reported in the original paper and follow the standard training procedure on these two tasks.

\paragraph{DeepFRI~\citep{gligorijevic2021structure}.} We also evaluate DeepFRI~\citep{gligorijevic2021structure} in our benchmark, which is a popular structure-based encoder for protein function prediction. DeepFRI employs an LSTM model to extract residue features and further constructs a residue graph to propagate messages among residues, in which a 3-layer graph convolutional network (GCN)~\citep{kipf2017semi} is used. We directly utilize the official model checkpoint for baseline evaluation. 

\paragraph{ESM-1b~\citep{rives2021biological}.} Besides the from-scratch sequence encoders above, we also compare with two state-of-the-art pretrained protein language models. ESM-1b~\citep{rives2021biological} is a huge Transformer encoder model whose size is larger than BERT-Large~\citep{devlin2018bert}, and it is pretrained on 24 million protein sequences from UniRef50~\citep{suzek2007uniref} by masked language modeling (MLM)~\citep{devlin2018bert}. In our evaluation, we finetune the ESM-1b model with the learning rate that is one-tenth of that of the MLP prediction head.

\paragraph{ProtBERT-BFD~\citep{elnaggar2020prottrans}.} The other protein language model evaluated in our benchmark is ProtBERT-BFD~\citep{elnaggar2020prottrans} whose size also excesses BERT-Large~\citep{devlin2018bert}. This model is pretrained on 2.1 billion protein sequences from BFD~\citep{steinegger2018clustering} by MLM~\citep{devlin2018bert}. The evaluation of ProtBERT-BFD uses the same learning rate configuration as ESM-1b.

\paragraph{LM-GVP~\citep{wang2021lm}.} To further enhance the effectiveness of GVP~\citep{jing2021equivariant}, ~\citet{wang2021lm} proposed to prepend a protein language model, \emph{i.e.} ProtBERT~\citep{elnaggar2020prottrans}, before GVP to additionally utilize protein sequence representations. We also adopt this hybrid model as one of our baselines, and its implementation follows the official source code.

\paragraph{Our methods.}
For pretraining, we use Adam optimizer with learning rate 0.001 and train a model for 50 epochs.
Then, the pretrained model will be finetuned on downstream datasets.

For \textbf{Multiview Contrast}, we set the cropping length of subsequence operation as 50, the radius of subspace operation as 15$\mathrm{\AA}$, the mask rate of random edge masking operation as 0.15.
The temperature $\tau$ in the InfoNCE loss function is set as 0.07.
When pretraining \method-Edge and \method-Edge-IEConv, we use 96 and 24 as batch sizes, respectively.

For \textbf{Distance Prediction}, we set the number of sampled residue pairs as 256.
The batch size will be set as 128 and 32 for \method-Edge and \method-Edge-IEConv, respectively.
For \textbf{Residue Type}, \textbf{Angle} and \textbf{Dihedral Prediction}, we set the number of sampled residues, residue triplets and residue quadrants as  512.
The batch size will be set as 96 and 32 for \method-Edge and \method-Edge-IEConv, respectively.

For downstream evaluation, the hidden representations in each layer of \method will be concatenated for the final prediction.
Table~\ref{tab:hyperparameter} lists the hyperparameter configurations for different downstream tasks.
For the four tasks, we use the same optimizer and number of epochs as in the original papers to make fair comparison.
For EC and GO prediction, we use ReduceLROnPlateau scheduler with factor $0.6$ and patience $5$, while we use StepLR scheduler with step size $50$ and gamma $0.5$ for fold and reaction classification.

\begin{table}[!t]
    \centering
    \caption{Hyperparameter configurations of our model on different datasets. The batch size reported in the table refers to the batch size on each GPU. All the hyperparameters are chosen by the performance on the validation set.}
    \label{tab:hyperparameter}
    \begin{adjustbox}{max width=0.6\linewidth}
        \begin{tabular}{llcccc}
            \toprule
            \multicolumn{2}{l}{\bf{Hyperparameter}}
            & \bf{EC} & \bf{GO} & \bf{Fold} & \bf{Reaction} \\
            \midrule
            \multirow{3}{*}{\bf{GNN}}
            & \#layer & 6 & 6 & 6 & 6\\
            & hidden dim. & 512 & 512 & 512 & 512 \\
            & dropout & 0.1 & 0.1 & 0.2 & 0.2 \\
            \midrule
            \multirow{5}{*}{\bf{Learning}}
            & optimizer     & Adam   & Adam   & SGD & SGD  \\
            & learning rate & 1e-4 & 1e-4 & 1e-3 & 1e-3 \\
            & weight decay & 0 & 0 & 5e-4     & 5e-4 \\
            & batch size & 2 & 2 & 2 & 2 \\
            % & scheduler     & ReduceLROnPlateau & ReduceLROnPlateau & StepLR & StepLR  \\
            & \# epoch & 200 & 200 & 300 & 300 \\
            
            \bottomrule
        \end{tabular}
    \end{adjustbox}
\end{table}

\section{Additional Experimental Results on EC and GO Prediction}
\label{sec:app_exp}

\paragraph{Results under different sequence identity cutoffs.}
% In the experiments above, we use $95\%$ cutoff for EC and GO prediction to make a fair comparison with LM-GVP.
Besides the experiments in Section~\ref{sec:exp}, where 95\% is used as the sequence identity cutoff for EC and GO dataset splitting, we also test our models and several important baselines under four lower sequence identity cutoffs and show the experimental results in Table~\ref{tab:seq_cutoff}.
The aim of this experiment is to test the robustness of different models under different hold-out test sets, with lowering cutoff indicating lower similarity between training and test sets.
It can be observed that, at lower cutoffs, our model can still achieve the best performance among models without pretraining and get comparable or better results against ESM-1b after pretraining.

\begin{table*}[t]
    \centering
    \caption{F\textsubscript{max} on EC and GO tasks under different sequence cutoffs (30\% / 40\% / 50\% / 70\% / 95\%).}
    \label{tab:seq_cutoff}
    \begin{adjustbox}{max width=\linewidth}
        \begin{tabular}{lcccc} %cccccccccccc
            \toprule
            \multirow{1}{*}{\bf{Method}}
            & \bf{EC} & \bf{GO-BP} & \bf{GO-MF} & \bf{GO-CC} \\
            % & \multicolumn{4}{c}{\bf{EC}} 
            % & \multicolumn{4}{c}{\bf{GO-BP}} & \multicolumn{4}{c}{\bf{GO-MF}} & \multicolumn{4}{c}{\bf{GO-CC}} \\
            % \cmidrule{2-17}
            % & 30\% & 40\% & 50\% & 70\% &
            % 30\% & 40\% & 50\% & 70\% &
            % 30\% & 40\% & 50\% & 70\% &
            % 30\% & 40\% & 50\% & 70\%\\
            \midrule
            \bf{CNN} & 0.366 / 0.361 / 0.372 / 0.429 / 0.545 & 0.197 / 0.195 / 0.197 / 0.211 / 0.244 & 0.238 / 0.243 / 0.256 / 0.292 / 0.354 & 0.258 / 0.257 / 0.260 / 0.263 / 0.387 \\
            \bf{ResNet} & 0.409 / 0.412 / 0.450 / 0.526 / 0.605 & 0.230 / 0.230 / 0.234 / 0.249 / 0.280 & 0.282 / 0.288 / 0.308 / 0.347 / 0.405 & 0.277 / 0.273 / 0.280 / 0.278 / 0.304 \\
            \bf{LSTM} & 0.247 / 0.249 / 0.270 / 0.333 / 0.425 & 0.194 / 0.192 / 0.195 / 0.205 / 0.225 & 0.223 / 0.229 / 0.245 / 0.276 / 0.321 & 0.263 / 0.264 / 0.269 / 0.270 / 0.283 \\
            \bf{Transformer} & 0.167 / 0.173 / 0.175 / 0.197 / 0.238 & 0.267 / 0.265 / 0.262 / 0.262 / 0.264 & 0.184 / 0.187 / 0.195 / 0.204 / 0.211 & 0.378 / 0.382 / 0.388 / 0.395 / 0.405 \\
            \bf{GCN} & 0.245 / 0.246 / 0.246 / 0.280 / 0.320 & 0.251 / 0.250 / 0.248 / 0.248 / 0.252 & 0.180 / 0.183 / 0.187 / 0.194 / 0.195 & 0.318 / 0.318 / 0.320 / 0.323 / 0.329\\
            \bf{GearNet} & 0.557 / 0.570 / 0.615 / 0.693 / 0.730 & 0.309 / 0.309 / 0.315 / 0.336 / 0.356 & 0.382 / 0.397 / 0.425 / 0.474 / 0.503 & 0.381 / 0.385 / 0.393 / 0.398 / 0.414\\
            \bf{GearNet-edge} & \bf{0.625} / \bf{0.646} / \bf{0.694} / \bf{0.757} / \bf{0.810} & \bf{0.345} / \bf{0.347} / \bf{0.354} / \bf{0.378} / \bf{0.403} & \bf{0.444} / \bf{0.461} / \bf{0.490} / \bf{0.537} / \bf{0.580} & \bf{0.394} / \bf{0.394} / \bf{0.401} / \bf{0.408} / \bf{0.450}\\
            \midrule
            \bf{DeepFRI} & 0.470 / 0.505 / 0.545 / 0.600 / 0.631 & 0.361 / 0.362 / 0.371 / 0.391 / 0.399 & 0.374 / 0.383 / 0.409 / 0.446 / 0.465 & 0.440 / 0.441 / 0.444 / 0.451 / 0.460\\
            \bf{ESM-1b} & 0.737 / 0.764 / 0.797 / 0.839 / 0.864 & 0.394 / 0.399 / 0.407 / 0.429 / 0.452 & \bf{0.546} / \bf{0.562} / \bf{0.588} / \bf{0.625} / \bf{0.657} & \bf{0.462} / \bf{0.465} / \bf{0.468} / 0.465 / \bf{0.477}\\
            % \bf{Residue Type Prediction} & 0.470 / 0.505 / 0.545 / 0.600 / 0.631 & 0.361 / 0.362 / 0.371 / 0.391 / 0.399 & 0.374 / 0.383 / 0.409 / 0.446 / 0.465 & 0.440 / 0.441 / 0.444 / 0.451 / 0.460\\
            % \bf{Distance Prediction} & 0.470 / 0.505 / 0.545 / 0.600 / 0.631 & 0.361 / 0.362 / 0.371 / 0.391 / 0.399 & 0.374 / 0.383 / 0.409 / 0.446 / 0.465 & 0.440 / 0.441 / 0.444 / 0.451 / 0.460\\
            % \bf{Angle Prediction} & 0.470 / 0.505 / 0.545 / 0.600 / 0.631 & 0.361 / 0.362 / 0.371 / 0.391 / 0.399 & 0.374 / 0.383 / 0.409 / 0.446 / 0.465 & 0.440 / 0.441 / 0.444 / 0.451 / 0.460\\
            % \bf{Dihedral Prediction} & 0.470 / 0.505 / 0.545 / 0.600 / 0.631 & 0.361 / 0.362 / 0.371 / 0.391 / 0.399 & 0.374 / 0.383 / 0.409 / 0.446 / 0.465 & 0.440 / 0.441 / 0.444 / 0.451 / 0.460\\
            \bf{Multiview Contrast} & \bf{0.744} / \bf{0.769} / \bf{0.808} / \bf{0.848} / \bf{0.874} & \bf{0.436} / \bf{0.442} / \bf{0.449} / \bf{0.471} / \bf{0.490} & 0.533 / 0.548 / 0.573 / 0.612 / \bf{0.654} & 0.459 / 0.460 / \bf{0.467} / \bf{0.469} / \bf{0.488}\\
            \bottomrule
        \end{tabular}
    \end{adjustbox}
\end{table*}

\paragraph{AUPR on EC and GO prediction.}
We have reported experimental results on EC and GO prediction with F\textsubscript{max} as the metric in Section~\ref{sec:exp}.
Here we report another popular metric AUPR in Table~\ref{tab:aupr}.
Note that we still use the best model selected by F\textsubscript{max} on validation sets.
It can be observed that our model can still achieve the best performance on EC prediction in both from scratch and pretrained settings.
However, there are still non-trivial gaps between our models with the state-of-the-art results.
This probably is because of the inconsistency between the two evaluation metrics.
It would be interesting to study the relationship between these two metrics and develop a model good at both in future works.

\begin{table*}[!t]
    \centering
    \caption{AUPR on EC and GO prediction. [\textdagger] denotes results taken from~\citet{wang2021lm}.
    For pretraining,
    we select the model with the best performance when training from scratch, \emph{i.e.}, \method-Edge. We omit the model name and use pretraining methods to name our pretrained models.
    }
    \label{tab:aupr}
    \begin{adjustbox}{max width=0.8\linewidth}
        \begin{tabular}{lcccccc}
            \toprule
            & \multirow{2}{*}{\bf{Method}} &
            \multirowcell{2}{\bf{Pretraining} \\\bf{Dataset (Size)}} &
            \multirow{2}{*}{\bf{EC}}&
            \multicolumn{3}{c}{\bf{GO}}\\
            \cmidrule{5-7}
            & & & & \bf{BP} & \bf{MF}& \bf{CC} \\
            \midrule
            \multirow{14}{*}{\rotatebox{90}{\bf{w/o pretraining}}}
            & CNN~\citep{shanehsazzadeh2020transfer} & - & 0.526& 0.159& 0.351& 0.204\\
            & ResNet~\citep{tape2019} & - & 0.590& 0.205& 0.434& 0.214\\
            & LSTM~\citep{tape2019} & - & 0.414& 0.156& 0.334& 0.192\\
            & Transformer~\citep{tape2019} & - & 0.218& 0.156& 0.177& 0.210\\
            \cmidrule{2-7}
            & GCN~\citep{kipf2017semi} & - & 0.319& 0.136& 0.147& 0.175\\
            & GAT~\citep{velickovic2018graph} & - & 0.320& 0.171\textsuperscript{\textdagger}& 0.329\textsuperscript{\textdagger}& 0.249\textsuperscript{\textdagger}\\
            & GVP~\citep{jing2021equivariant} & - & 0.482& 0.224\textsuperscript{\textdagger}& 0.458\textsuperscript{\textdagger}& 0.279\textsuperscript{\textdagger}\\
            & 3DCNN\_MQA~\citep{derevyanko2018deep} & - & 0.029&0.132& 0.075& 0.144\\
            & GraphQA~\citep{baldassarre2021graphqa}  & - & 0.543& 0.199& 0.347& 0.265\\
            % & IEConv~\cite{hermosilla2020intrinsic} & - & -& -& -& -\\
            & New IEConv~\citep{anonymous2022contrastive} & - & 0.775& \bf{0.273}& \bf{0.572}& \bf{0.316}\\
            \cmidrule{2-7}
            & \textbf{\method} & - & 0.751& 0.211& 0.490& 0.276\\
            & \textbf{\method-IEConv} & - & 0.835 & 0.231& 0.547 & 0.259  \\
            & \textbf{\method-Edge} & - & 0.835&0.251& \bf{0.570}& 0.303\\
            & \textbf{\method-Edge-IEConv} & - & \bf{0.843}   &  0.244   & 0.561   & 0.284  \\
            \midrule
            \multirow{9}{*}{\rotatebox{90}{\bf{w/ pretraining}}}
            & DeepFRI~\citep{gligorijevic2021structure} & Pfam (10M) & 0.547& 0.282& 0.462& 0.363\\
            & ESM-1b~\citep{rives2021biological} & UniRef50 (24M) & 0.889& \bf{0.332}& \bf{0.639}& 0.324\\
            & ProtBERT-BFD~\citep{elnaggar2020prottrans}  & BFD (2.1B) & 0.859& 0.188\textsuperscript{\textdagger}& 0.464\textsuperscript{\textdagger}& 0.234\textsuperscript{\textdagger}\\
            & LM-GVP~\citep{wang2021lm} & UniRef100 (216M) & 0.710& 0.302\textsuperscript{\textdagger}& 0.580\textsuperscript{\textdagger}& \bf{0.423\textsuperscript{\textdagger}}\\
            \cmidrule{2-7}
            & {Residue Type Prediction} & AlphaFoldDB (805K) & 0.870& 0.267& 0.583& 0.311 \\
            & {Distance Prediction} & AlphaFoldDB (805K) & 0.863& 0.274& 0.586& 0.327\\
            & {Angle Prediction} & AlphaFoldDB (805K) & 0.880& 0.291& 0.603& 0.331\\
            & {Dihedral Prediction}  & AlphaFoldDB (805K) & 0.881& 0.304& 0.603& 0.338\\
            \cmidrule{2-7}
            & \textbf{Multiview Contrast} & AlphaFoldDB (805K) & \bf{0.892}& 0.292& 0.596& 0.336\\
            \bottomrule
        \end{tabular}
    \end{adjustbox}
\end{table*}

\paragraph{Sampling schemes in self-prediction methods.}
Different sampling schemes may lead to different results for self-prediction methods.
We study the effects of sampling schemes using Dihedral Prediction as an example.
Instead of sampling dihedral angles formed by three consecutive edges, we try to predict the dihedrals formed by four randomly sampled nodes.
We observe that the F\textsubscript{max} decreases from $0.859$ to $0.821$.
This suggests that it is better of learning residue representations to capture local spatial information instead of global  information.
The change of sampling schemes will make self-prediction tasks more difficult to solve, which even brings negative effects after pretraining.

\paragraph{Pretraining on different datasets.}
We use the AlphaFold protein structure database as our pretraining database, because it contains the largest number of protein structures and is planned to cover over 100 million proteins.
However, the structures in this database are not experimentally determined but predicted by AlphaFold2.
Therefore, it is interesting to see the performance of our methods when pretraining on different datasets. 

To study the effects of the choice of pretraining dataset, we build another dataset using structures extracted from Protein Data Bank (PDB)~\citep{berman2000protein}.
Specifically, we extract 123,505 experimentally-determined protein structures from PDB whose resolutions are between 0.0 and 2.5 angstroms, and we further extract 305,265 chains from these proteins to construct the final dataset. 
% Describe the details of dataset construction\textcolor{red}{@Minghao}.

Next, we pretrain our five methods on AlphaFold Database v1 (proteome-wide structure predictions), AlphaFold Database v2 (Swiss-Prot structure predictions) and Protein Data Bank and then evaluate the pretrained models on the EC prediction task.
The results are reported in Table~\ref{tab:pretrain_dataset}.
As can be seen in the table, our methods can achieve comparable performance on different pretraining datasets.
Consequently, our methods are robust to the choice of pretraining datasets.
\begin{table*}[!t]
    \centering
    \caption{Results of \method-Edge pretrained on different pretraining datasets with different methods. 
    Models are evaluated on the EC prediction task.}
    \label{tab:pretrain_dataset}
    \begin{adjustbox}{max width=\linewidth}
        %\footnotesize
        \begin{tabular}{lcccccccccccccccc}
            \toprule
            \multirow{2}{*}{\bf{Dataset}} &
            \multirow{2}{*}{\bf{\# Proteins}} & &
            \multicolumn{2}{c}{\bf{Multivew Contrast}}
            & &
            \multicolumn{2}{c}{\bf{Residue Type Prediction}}
            & &
            \multicolumn{2}{c}{\bf{Distance Prediction}}
            & &
            \multicolumn{2}{c}{\bf{Angle Prediction}}
            & &
            \multicolumn{2}{c}{\bf{Dihedral Prediction}}\\
            \cmidrule{4-5}
            \cmidrule{7-8}
            \cmidrule{10-11}
            \cmidrule{13-14}
            \cmidrule{16-17}
            & & & \bf{AUPR\textsubscript{pair}} & \bf{F\textsubscript{max}}
            & & \bf{AUPR\textsubscript{pair}} & \bf{F\textsubscript{max}}
            & & \bf{AUPR\textsubscript{pair}} & \bf{F\textsubscript{max}}
            & & \bf{AUPR\textsubscript{pair}} & \bf{F\textsubscript{max}}
            & & \bf{AUPR\textsubscript{pair}} & \bf{F\textsubscript{max}}\\
            \midrule
            \bf{AlphaFold Database (v1 + v2)} & 804,872 && 0.892 & 0.874 && 0.870 & 0.834&& 0.863 & 0.839 && 0.880 & 0.853 && 0.881 & 0.859 \\
            \bf{AlphaFold Database (v1)} & 365,198 && 0.890 & 0.874 && 0.869& 0.842 && 0.871 & 0.843 && 0.879 & 0.854 && 0.877 & 0.852 \\
            \bf{AlphaFold Database (v2)} & 439,674 && 0.890 & 0.874 && 0.868& 0.838&& 0.868 & 0.846 && 0.881 & 0.853 && 0.883 & 0.861 \\
            \bf{Protein Data Bank} & 305,265 && 0.881 & 0.859 && 0.870& 0.841&& 0.865& 0.847&& 0.880 & 0.857 && 0.886 & 0.858\\
            \bottomrule
        \end{tabular}
    \end{adjustbox}
\end{table*}

\section{\textcolor{red}{Structure Pretraining on EGNN}}
\label{sec:egnn}
\begin{wraptable}{R}{0.35\textwidth}
\begin{minipage}[t]{\linewidth}
\vspace{-2em}
    \begin{adjustbox}{max width=\linewidth}
        \footnotesize
        \begin{tabular}{cc}
            \toprule
            \bf{Method}  & \bf{F\textsubscript{max}}\\
            \midrule
            \bf{EGNN}   & 0.640 \\
            \midrule
            Residue Type Prediction&0.729 \\
            Distance Prediction&\bf{0.761}\\
            Angle Prediction&0.718\\
            Dihedral Prediction&0.662\\
            \midrule
            \bf{Multiview Contrast} & 0.752\\
            \bottomrule
        \end{tabular}
    \end{adjustbox}
    \caption{\textcolor{red}{Pretraining results on EC with EGNN as backbone models.}}
    \label{tab:backbone}
    \vspace{-1.5em}
\end{minipage}%
\end{wraptable}

\textcolor{red}{
To verify the effectiveness of our proposed  methods, we choose another common backbone model, equivariant graph neural network (EGNN)~\citep{satorras2021n}, for pretraining.
We follow the experimental setup in Appendix~\ref{sec:app_impl} for pretraining and finetuning the model.
The results on the EC dataset are reported in Table~\ref{tab:backbone}.
It can be seen that the performance of the EGNN is improved by a large margin with all the five pretraining methods.
Among them, Distance Prediction and Multiview Contrast are the top two methods. 
The ranks of these five methods are quite different from the ranks in the main paper.
This is probably because the capacity of EGNN limits its performance on some pretraining tasks and thus reduces their benefits.
}

\section{\textcolor{red}{Combine Sequence- and Structure-Based Encoders}}
\label{sec:seq_struct}
\begin{wraptable}{R}{0.45\textwidth}
\begin{minipage}[t]{\linewidth}
\vspace{-1em}
\begin{adjustbox}{max width=\linewidth}
        \begin{tabular}{lcccc}
            \toprule
            \multirow{2}{*}{\bf{Method}}  &
            \multirow{2}{*}{\bf{EC}}&
            \multicolumn{3}{c}{\bf{GO}}\\
            \cmidrule{3-5}
            & & \bf{BP} & \bf{MF}& \bf{CC}\\
            \midrule
            \method & 0.730& 0.356& 0.503& 0.414\\
            \method-Edge & 0.810&0.403& 0.580& 0.450\\
            {\footnotesize -w/ Multiview Contrast} & 0.874& 0.490& 0.654& 0.488\\
            \midrule
            ESM-1b & 0.864& 0.452& 0.657& 0.477\\
            \midrule
            \textbf{ESM-1b+GearNet} & \bf{0.883}& \bf{0.491}& \bf{0.677}& \bf{0.501}\\
            % \textbf{{\footnotesize -w/ Multiview Contrast}} & \bf{0.894}& \bf{0.516}& \bf{0.684}& \bf{0.506}\\
            \bottomrule
        \end{tabular}
    \end{adjustbox}
    \caption{\textcolor{red}{Results (F\textsubscript{max}) for combining seuqence- and structure-based encoders.}
    }
    \label{tab:esm_gearnet}
    \vspace{-1em}
\end{minipage}%
\end{wraptable}
\textcolor{red}{
In the main paper, we compare the pretrained sequence- and structure-based encoder and show that geometric structure pretraining can achieve competitive results with much less  data.
To further show the benefit of incorporating structural information, here we choose ESM-1b as a baseline and build a structure-based encoder based on its output.
Specifically, we replace the raw node features in \method with pretrained sequence representations.
We train the model on EC with the same configurations for \method and finetune the ESM-1b model with learning rate 1e-5.
The results are shown in Table~\ref{tab:esm_gearnet}.
It can be observed that the ESM-1b+GearNet model can achieve SOTA performance even without structure-based pretraining, which suggests the importance of utilizing protein structures.
Also, it is promising to explore pretraining methods on the combined encoder.
We leave this direction for future work.
}

\section{\textcolor{red}{Combine Neural and Retrieval-Based Methods}}
\label{sec:retrieval}
\textcolor{red}{
Searching a database to retrieve similar proteins is a popular method used in the biological community when predicting properties of a target protein, \emph{e.g.}, searching multiple sequence alignments and templates for structure prediction~\citep{jumper2021highly}.
There have been a large amount of tools proposed for aligning protein sequences~\citep{Altschul1997GappedBA,Steinegger2017MMseqs2ES,Steinegger2019HHsuite3FF} and structures~\citep{Yang2006ProteinSD,Zhang2005TMalignAP,vanKempen2022FoldseekFA,Holm2019BenchmarkingFD}.
In this section, we first compare our neural representation-based method with retrieval-based methods on function and fold classification tasks and then showcase the potential of our proposed methods on structure-based search tasks.
}

\begin{table*}[!h]
    \centering
    \begin{adjustbox}{max width=\linewidth}
        %\footnotesize
        \begin{tabular}{lcccccccccccccccc}
            \toprule
            \multirow{2}{*}{\bf{Method}} &
            \multicolumn{2}{c}{\bf{EC}}
            & &
            \multicolumn{2}{c}{\bf{GO-BP}}
            & &
            \multicolumn{2}{c}{\bf{GO-MF}}
            & &
            \multicolumn{2}{c}{\bf{GO-CC}}
            &&
            \multicolumn{4}{c}{\bf{Fold Classification}}
            \\
            \cmidrule{2-3}
            \cmidrule{5-6}
            \cmidrule{8-9}
            \cmidrule{11-12}
            \cmidrule{14-17}
            & \bf{AUPR\textsubscript{pair}} & \bf{F\textsubscript{max}}
            & & \bf{AUPR\textsubscript{pair}} & \bf{F\textsubscript{max}}
            & & \bf{AUPR\textsubscript{pair}} & \bf{F\textsubscript{max}}
            & & \bf{AUPR\textsubscript{pair}} & \bf{F\textsubscript{max}}
            & & \bf{Fold} & \bf{Super.} & \bf{Fam.} & \bf{Avg.}\\
            \midrule
            Foldseek~\citep{vanKempen2022FoldseekFA} & 0.778 & 0.888 && 0.168 & 0.440 && 0.462 & 0.649 && 0.159 & 0.321 && 2.78 & 7.57 & 65.4& 25.2\\
            \midrule
            \bf{\method-Edge(-IEConv)} & 0.835 & 0.810 && 0.251 & 0.403&& 0.570 & 0.580 && 0.303 & 0.450 && 48.3 & 70.3 & 99.5 & 72.7 \\
            \bf{\footnotesize w/ Multiview Contrast} & 0.892 & 0.874 && 0.292 & 0.490&& 0.596 & 0.654 && \bf{0.336} & \bf{0.488} && \bf{54.1} & \bf{80.5} & \bf{99.9} & \bf{78.1}\\
            % \midrule
            \bf{\footnotesize w/ Multiview Contrast + Foldseek} & \bf{0.908} & \bf{0.903} && \bf{0.314} & \bf{0.500} && \bf{0.615} & \bf{0.673} && 0.319 & 0.467 && - & - & - & -\\
            \bottomrule
        \end{tabular}
    \end{adjustbox}
    \caption{\textcolor{red}{Comparison between neural and retrieval-based methods on EC, GO and fold classification tasks. As in Table~\ref{tab:all_result}, we use \method-Edge on EC and GO prediction and \method-Edge-IEConv on fold classification as backbone models. The results w/o and w/ pretraining and those ensembled with Foldseek are reported on EC and GO. We omit the ensemble results on fold classification due to the poor performance of Foldseek.}}
    \label{tab:retrieval}
\end{table*}

\textcolor{red}{
\paragraph{Comparison with retrieval-based methods.}
We select a structure alignment tool, Foldseek~\citep{vanKempen2022FoldseekFA}, as our retrieval-based baseline.
The method trains a VQ-VAE on SCOPe40 to discretize  structural units into an alphabet of twenty 3Di states and then transforms the problem to 3Di sequence alignment, which is done by MMseqs2~\citep{Steinegger2017MMseqs2ES}.
When using Foldseek, we follow the parameters provided in their github repo\footnote{https://github.com/steineggerlab/foldseek-analysis/blob/main/scopbenchmark/scripts/runFoldseek.sh}.
For each protein in the test set of our benchmark tasks, we use Foldseek to retrieve the most similar protein in the training set, the label of which will be used for prediction.
}

\textcolor{red}{
We report the results of retrieval-based and our proposed neural methods in Table~\ref{tab:retrieval}.
First, we find that Foldseek achieves very good performance on EC and GO prediction.
In terms of F\textsubscript{max}, it is better than \method-Edge on all tasks and competitive with the pretrained \method-Edge on EC and GO-MF.
The accuracy of Foldseek makes it a strong baseline for proteins with similar structures in the training set.
However, when the dataset is split by structural similarities, \emph{e.g.}, fold classification, the structural alignment tool fails to retrieve similar proteins and get accurate prediction as shown in the table.
This can be attributed to the inherent limitation of retrieval-based methods, \emph{i.e.}, the lack of generalization ability to novel data points.
}

\textcolor{red}{
Furthermore, to utilize the advantages from both worlds, we combine neural and retrieval-based methods via ensemble.
As shown in the last row of Table~\ref{tab:retrieval}, both metrics are significantly improved on EC, GO-BP, GO-MF compared with the separate neural and retrieval-based methods.
Consequently, it would be interesting to explore the combination of these two kinds of methods in the future, as have done in many machine learning tasks~\citep{Mitra2017NeuralMF,Sun2019PullNetOD,Notin2022TranceptionPF}. 
}

\textcolor{red}{
\paragraph{Results on structure-based search tasks.}
To show the potential of structure-based modeling for biological applications, we test our model on the SCOPe40 benchmark proposed in~\citet{vanKempen2022FoldseekFA}.
The authors cluster the SCOPe 2.0198 at 40\% sequence identity and obtain 11,211 non-redundant protein sequences.
They perform an all-versus-all search on the dataset and test the ability of structure alignment tools for finding proteins of the same SCOPe family, superfamily, and fold.
For each query, they measure the fraction of TPs (true positive matches) out of all correct matches until the first FP (false positive) that matches to a different fold.
The sensitivity is calculated by the area under the curve of the cumulative ROC curve up to the first FP.
}

\begin{table*}[h]
    \centering
    \caption{\textcolor{red}{Sensitivity of searching proteins of the same family, superfamily and fold on SCOPe40. Results are evaluated with the scripts and predictions provided in~\citep{vanKempen2022FoldseekFA}.}}
    \label{tab:scop}
    \begin{adjustbox}{max width=\linewidth}
        %\footnotesize
        \begin{tabular}{lcccc}
            \toprule
            \bf{Method} &
            \bf{Fold} & \bf{Super.} & \bf{Fam.} & \bf{Avg.}
            \\
            \midrule
            MMseqs2~\citep{Steinegger2017MMseqs2ES} & 0.001 & 0.082 & 0.542 & 0.208\\
            3D-BLAST~\citep{Yang2006ProteinSD} & 0.009 & 0.126 & 0.572 & 0.235\\
            CLE-SW~\citep{Zhao2013SSWLA} & 0.021 & 0.293 & 0.763 & 0.359\\
            CE~\citep{Shindyalov1998ProteinSA} & 0.131 & 0.529 & 0.885 & 0.515\\
            TMalign-fast~\citep{Zhang2005TMalignAP} & 0.188 & 0.618 & 0.906 & 0.571\\
            TMalign~\citep{Zhang2005TMalignAP} & 0.188 & 0.610 & 0.901 & 0.566\\
            Foldseek~\citep{vanKempen2022FoldseekFA} & 0.155 & 0.593 & 0.914 & 0.554\\
            DALI~\citep{Holm2019BenchmarkingFD} & 0.310 & 0.751 & 0.942 & 0.667\\
            \midrule
            \bf{\method-Edge-IEConv} & 0.474 & 0.722 & 0.936 & 0.710\\
            \midrule
            \bf{\method-Edge-IEConv + DALI} & \bf{0.481}& \bf{0.779}& \bf{0.963}& \bf{0.741} \\
            \bottomrule
        \end{tabular}
    \end{adjustbox}
\end{table*}

\textcolor{red}{
We report the results of seven structure alignment tools and a sequence search tool evaluated in~\citet{vanKempen2022FoldseekFA}.
For comparison, we use the \method-Edge-IEConv model trained on fold classification to extract representations for proteins and use the cosine similarity between representations to retrieve similar proteins.
The sensitivity of these methods is reported in Table~\ref{tab:scop}.
It can be observed that our method achieves the best performance on average among all baselines.
Compared with DALI, though finding fewer proteins of the same family and superfamily, our method can achieve higher sensitivity at the fold level.
This can be explained by the better generalization ability to novel structures of neural methods.
With the ensemble of neural and retrieval-based methods, we can achieve the SOTA performance at all levels.
This again demonstrates the effectiveness of our proposed method and the potential of combining neural and retrieval-based methods.
}

\section{Latent Space Visualization}
\label{sec:app_vis}

\begin{figure*}[t]
    \centering
    \includegraphics[width=0.9\linewidth]{figures/embedding.png}
    \caption{Latent space visualization of \method-Edge (Multiview Contrast) on AlphaFold Database v1.}
    \label{fig:embedding}
\end{figure*}

%%%%%%%%%%%%%%%%%%%%%%%%%%%%%%%%%%

For qualitatively evaluating the quality of the protein embeddings learned by our pretraining method, we visualize the latent space of the \method-Edge model pretrained by Multiview Contrast. Specifically, we utilize the pretrained model to extract the embeddings of all the proteins in AlphaFold Database v1, and these embeddings are mapped to the two-dimensional space by UMAP~\citep{mcinnes2018umap} for visualization. Following \citet{akdel2021structural}, we highlight the 20 most common superfamilies within the database by different colors. The visualization results are shown in Fig.~\ref{fig:embedding}. It can be observed that our pretrained model tends to group the proteins from the same superfamily together and divide the ones from different superfamilies apart. In particular, it succeeds in clearly separating three superfamilies, \emph{i.e.}, Protein kinase superfamily, Cytochrome P450 family and TRAFAC class myosin-kinesin ATPase superfamily. Such a decent capability of discriminating protein superfamilies, to some degree, interprets our model's superior performance on Fold Classification. 

%%%%%%%%%%%%%%%%%%%%%%%%%%%%%%%%%%

\section{Residue-Level Explanation}
\label{sec:app_explanation}

Protein functions are often reflected by specific regions on the 3D protein structures.
For example, the binding ability of a protein to a ligand is highly related to the binding interface between them.
Hence, to better interpret our prediction, we apply Integrated Gradients (IG)~\citep{sundararajan2017axiomatic}, a model-agnostic attribution method, on our model to obtain residue-level interpretation.
Specifically, we first select two molecular functions, ATP binding (GO:0005524) and Heme binding (GO:0020037), from GO terms that are related to ligand binding.
For each functional term, we pick one protein and feed it into the best model trained on the GO-MF dataset.
Then, we use IG to generate the feature attribution scores for each protein.
The method will integrate the gradient along a straight-line path between a baseline input and the original input.
Here the original input and baseline input are the node feature $\vf$ and a zero vector, respectively.
The final attribution score for each protein will be obtained by summing over the feature dimension.
The normalized score distribution over all residues are visualized in Figure~\ref{fig:bind}.
As can be seen, our model is able to identify the active sites around the ligand, which are likely to be responsible for binding.
Note that these attributions are directly generated from our model without any supervision, which suggests the decent interpretability of our model.

\begin{figure*}[t]
    \centering
    \includegraphics[width=0.8\linewidth]{figures/binding.png}
    \caption{Identification of active sites on proteins responsible for binding based on attribution scores.
    Two proteins binding to specific targets are selected for illustration (1NYR-A for ATP binding and 1B85-A for Heme binding).
    For these two complexes, ligands are shown in yellow spheres while the residues of the receptors are colored based on attribution scores.
    Residues with higher attribution scores are colored in red while those with lower scores are colored in blue.
}
    \label{fig:bind}
\end{figure*}
